# Supplementary material for: Coffee-Gym: An Environment for Evaluating and Improving Natural Language Feedback on Erroneous Code
Source: arXiv:2409.19715 source file (2024-10-04)
Supplement: Supplementary file 1 [file k_analysis.tex]

\begin{table}[t]
    \centering
    \small
    \resizebox{\columnwidth}{!}{
    \begin{tabular}{lccccc}

    \toprule
    \textbf{\textit{K}} & 1 & 3 & 5 & 7 & 9  \\ 
    \midrule
    \textbf{Pass@1} & 45.9 & 48.7 & \textbf{51.2} & 49.4 & 48.1 \\
    \bottomrule
    \end{tabular}
    }
    \caption{
        Anaylsis of diverse number of sampling $K$.
    }
    \label{tab:k_analysis}
\end{table}
